# Supplementary material for: Enhanced Mid-Photospheric Heating Around a Solar Pore
Source: arXiv:2611.12121 source file (2026-11-12)
Supplement: Supplementary file 1 [file appendix_table.tex]

\begin{table}[]
  \caption{Mean values and standard deviations of the observed continuum intensity and inferred atmospheric parameters, calculated from all valid pixels aggregated over the three rasters. The standard deviations describe the pixel-to-pixel dispersion within each region and do not represent uncertainties on the mean.}
  \label{tab:mean_parameters}
  \centering
  \begin{tabular}{lccccc}
    \colhead{Parameter} & \colhead{$\log\tau_{500}$} & \colhead{UM} & \colhead{UBF} & \colhead{QS} & \colhead{PB} \\
    %
    \hline
    %
               & $0$    & 5.08$\pm$0.13 & 5.56$\pm$0.18 & 6.35$\pm$0.18 & 6.38$\pm$0.17 \\
    $T$ {[kK]} & $-2$   & 4.36$\pm$0.15 & 4.52$\pm$0.20 & 4.83$\pm$0.16 & 5.18$\pm$0.16 \\
               & $-4.5$ & 7.86$\pm$0.42 & 8.04$\pm$0.57 & 7.58$\pm$0.84 & 7.38$\pm$0.86 \\
    %
    \hline
    %
                           & $0$    & 0.33$\pm$0.24 & 0.19$\pm$0.73 & 0.57$\pm$1.22  & 1.35$\pm$1.51 \\
    $v_{\rm los}$ {[km\,s$^{-1}$]} & $-2$   & 0.13$\pm$0.85 & 0.08$\pm$1.03 & -0.31$\pm$0.63 & -0.36$\pm$1.01 \\
                           & $-4.5$ & 0.50$\pm$1.28 & 0.47$\pm$1.32 & 0.67$\pm$1.58  & 0.99$\pm$2.52 \\
    %
    \hline
    %
                         & $0$    & -1.98$\pm$0.19 & -1.73$\pm$0.31 & -0.21$\pm$0.40 & -0.78$\pm$0.44 \\
    $B_{\rm los}$ {[kG]} & $-2$   & -1.48$\pm$0.14 & -1.27$\pm$0.27 & -0.18$\pm$0.34 & -0.43$\pm$0.41 \\ 
                         & $-4.5$ & -0.24$\pm$0.18 & -0.26$\pm$0.20 & -0.13$\pm$0.14 & -0.25$\pm$0.15 \\
    \hline
    %
                          & $0$    & 0.95$\pm$0.16 & 1.18$\pm$0.22 & 0.40$\pm$0.37 & 0.73$\pm$0.32 \\
    $B_{\rm perp}$ {[kG]} & $-2$   & 0.53$\pm$0.22 & 0.68$\pm$0.25 & 0.48$\pm$0.27 & 0.89$\pm$0.31 \\ 
                          & $-4.5$ & 0.36$\pm$0.13 & 0.41$\pm$0.13 & 0.39$\pm$0.14 & 0.55$\pm$0.15 \\
    %
    \hline
    %
    $I_{\rm cont}$ {[$10^{-5}$ erg\,cm$^{-2}$\,s$^{-1}$\,sr$^{-1}$\,Hz$^{-1}$]} &  & 2.23$\pm$0.14 & 2.87$\pm$0.24 & 4.11$\pm$0.27 & 4.21$\pm$0.25 \\
    %
  \end{tabular} 
\end{table}
